# Supplementary material for: Gauntlet: Finding Bugs in Compilers for Programmable Packet Processing
Source: arXiv:2006.01074 source file (2020-10-25)
Supplement: Supplementary file 1 [file aec_appendix.tex]

\newpage
\appendix
\section{Artifact Appendix}

%%%%%%%%%%%%%%%%%%%%%%%%%%%%%%%%%%%%%%%%%%%%%%%%%%%%%%%%%%%%%%%%%%%%%
\subsection{Abstract}
\toolname is a set of tools designed to find bugs in compilers for programmablet packet-processing devices. More precisely, \toolname targets the P4\textsubscript{16} language ecosystem and the P4\textsubscript{16} reference compiler~\cite{p416}.

\subsection{Artifact check-list}

{\small
\begin{itemize}
  \item {\bf Run-time environment: } Ubuntu 18.04 LTS
  \item {\bf Public link: } \projecturl
  \item {\bf Code licenses: }  Apache-2.0 License
\end{itemize}}

%%%%%%%%%%%%%%%%%%%%%%%%%%%%%%%%%%%%%%%%%%%%%%%%%%%%%%%%%%%%%%%%%%%%%
\subsection{Description}
The goal is to ensure that a P4 compiler correctly translates a given input P4 program to its target-specific binary. The compiler must not crash and preserve the semantics of the program as originally written. The suite has three major components:
\begin{itemize}
    \item \textbf{Bludgeon}, a fuzz tester that generates random P4 programs using libraries from \pfourc.
    \item \textbf{Translation Validation}, which analyzes the intermediate representation of a program after each compiler pass and identifies potential discrepancies. We support translation validation for the open-source \pfourc compiler front- and mid-end libraries
    \item \textbf{Model-based Testing}, which infers input and and corresponding output for a particular P4 program and generates end-to-end test packets. We have currently implemented model-based testing for the \bmv simple-switch~\cite{bmv2} and the Tofino hardware switch~\cite{tofino}.
\end{itemize}

%%%%%%%%%%%%%%%%%%%%%%%%%%%%%%%%%%%%%%%%%%%%%%%%%%%%%%%%%%%%%%%%%%%%%
\subsection{Installation}
Please see the \texttt{README} at \url{https://github.com/p4gauntlet/gauntlet} for instructions on how to install and use Gauntlet. 

%%%%%%%%%%%%%%%%%%%%%%%%%%%%%%%%%%%%%%%%%%%%%%%%%%%%%%%%%%%%%%%%%%%%%
\subsection{Evaluation and expected result}
The bugs we have collected can be found in the \texttt{bugs} folder of the main repository at \url{https://github.com/p4gauntlet/gauntlet}. The \texttt{README} will provide further info on the details of individual bugs and how to reproduce them.

%%%%%%%%%%%%%%%%%%%%%%%%%%%%%%%%%%%%%%%%%%%%%%%%%%%%%%%%%%%%%%%%%%%%%
\subsection{AE Methodology}

Submission, reviewing and badging methodology:\\
\url{https://www.usenix.org/conference/osdi20/call-for-artifacts}
